# Supplementary material for: Pressure-induced structural transformation of clathrate Ge$_{136}$ via an ultrafast recrystallization of an amorphous intermediate
Source: arXiv:2112.12486 ancillary file (2021-12-23)
Supplement: Supplementary file 1 [file supp_mat.pdf]

# Pressure-induced structural transformation of clathrate $Ge_{136}$ via an ultrafast recrystallization of an amorphous intermediate
## *Supplemental Material*

Marián Ryník,[1,*] Stefano Leoni,[2,†] and Roman Martoňák[1,‡]

[1] *Department of Experimental Physics, Comenius University, Mlynská Dolina F2, 842 48 Bratislava, Slovakia*
[2] *School of Chemistry, Cardiff University, Cardiff, CF10 3AT, UK*

(Dated: December 23, 2021)

## COMPUTATIONAL METHODS

Ab initio calculations were performed by the VASP code[1, 2] employing PBE functional[3], standard PAW pseudopotential with 4 valence electrons and cutoff of 226 eV. MD was performed with $2 \times 2 \times 2$ Monkhorst-Pack mesh of k-points[4] and time step of 2 fs. In NPT MD the barostat mass was set to 5000 a. u. Metadynamics simulations were performed by means of 0.5 ps NVT runs and Gaussian width and height were set to 60 (kbar $\AA^3)^{\frac{1}{2}}$ and 3600 kbar $\AA^3$, respectively. Simulation cell was formed by a single unit cell of $Ge_{136}$. In simulations we also used the ASE library[5]. For analysis of data we used the R.I.N.G.S. code [6], for preparation of some graphs the Plotly package [7] and figures of atomic configurations were produced using the OVITO package[8].

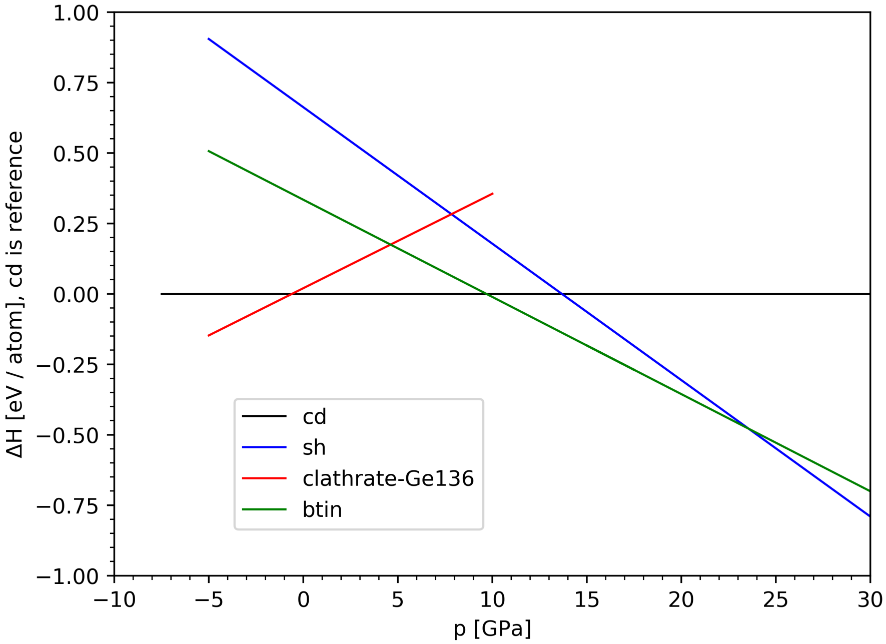


FIG. 1. Enthalpy (relative to the cubic diamond phase) as function of pressure for the $Ge_{136}$ clathrate, cubic diamond, $\beta$-tin and simple hexagonal phases.

* rynik@fmph.uniba.sk
† LeoniS@cardiff.ac.uk
‡ martonak@fmph.uniba.sk

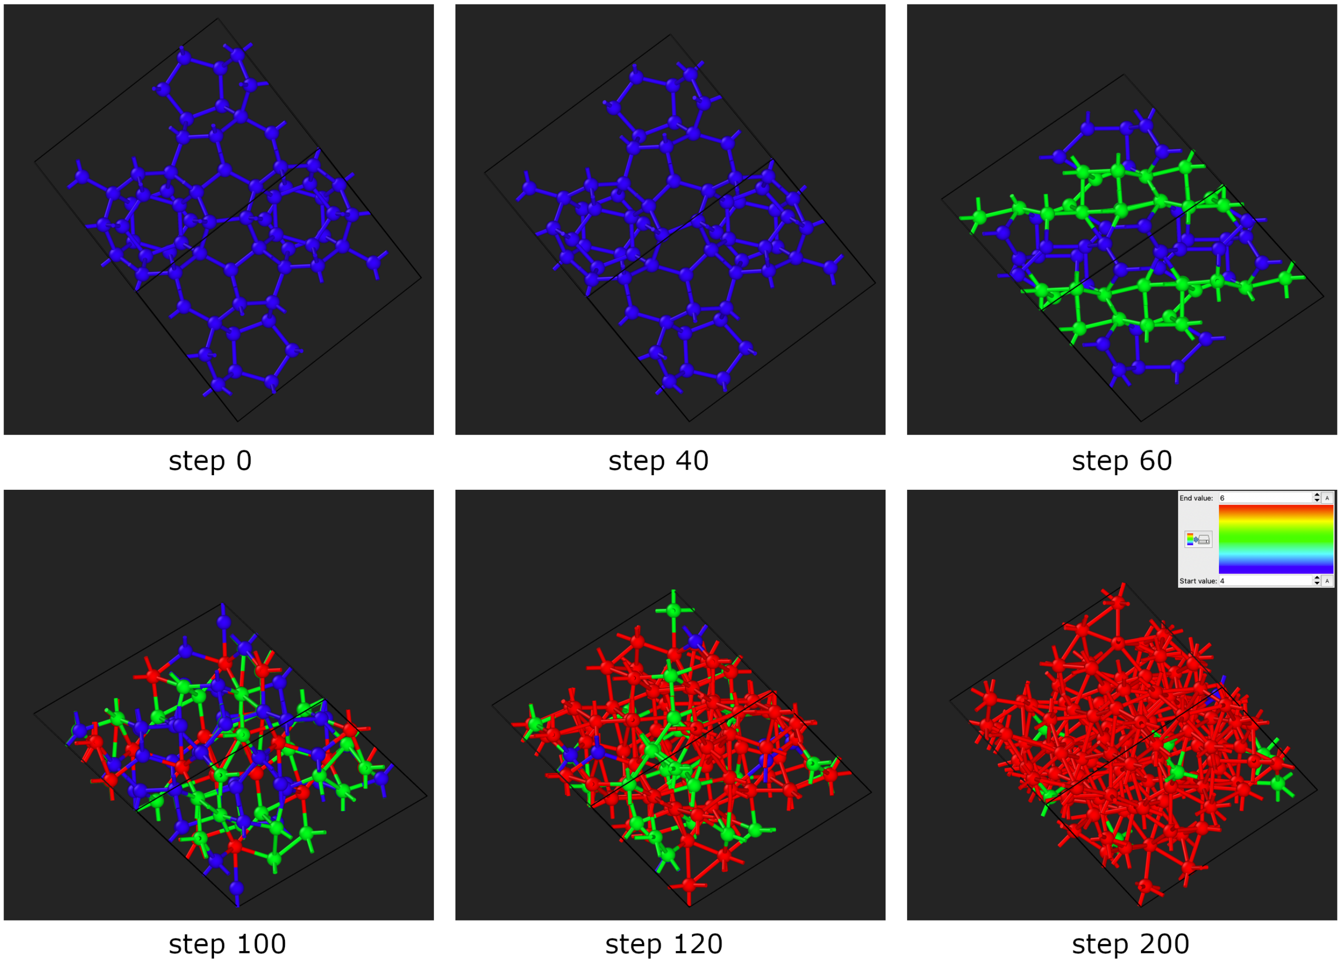


FIG. 2. Structural evolution during static compression of the clathrate $Ge_{136}$ at $p = 350$ kbar. Color represents coordination number of the atoms according to the colour map.


[1] G. Kresse and J. Furthmüller, Phys. Rev. B **54**, 11169 (1996).

[2] G. Kresse and D. Joubert, Phys. Rev. B **59**, 1758 (1999).

[3] J. P. Perdew, K. Burke, and M. Ernzerhof, Phys. Rev. Lett. **77**, 3865–3868 (1996).

[4] H. J. Monkhorst and J. D. Pack, Phys. Rev. B **13**, 5188 (1976).

[5] A. H. Larsen, J. J. Mortensen, J. Blomqvist, I. E. Castelli, R. Christensen, M. Dułak, J. Friis, M. N. Groves, B. Hammer, C. Hargus, E. D. Hermes, P. C. Jennings, P. B. Jensen, J. Kermode, J. R. Kitchin, E. L. Kolsbjerg, J. Kubal, K. Kaasbjerg, S. Lysgaard, J. B. Maronsson, T. Maxson, T. Olsen, L. Pastewka, A. Peterson, C. Rostgaard, J. Schiøtz, O. Schütt, M. Strange, K. S. Thygesen, T. Vegge, L. Vilhelmsen, M. Walter, Z. Zeng, and K. W. Jacobsen, Journal of Physics: Condensed Matter **29**, 273002 (2017).

[6] S. Le Roux and P. Jund, Computational Materials Science **49**, 70 (2010).

[7] P. T. Inc., "Collaborative data science," (2015).

[8] A. Stukowski, MODELLING AND SIMULATION IN MATERIALS SCIENCE AND ENGINEERING **18** (2010), 10.1088/0965-0393/18/1/015012.

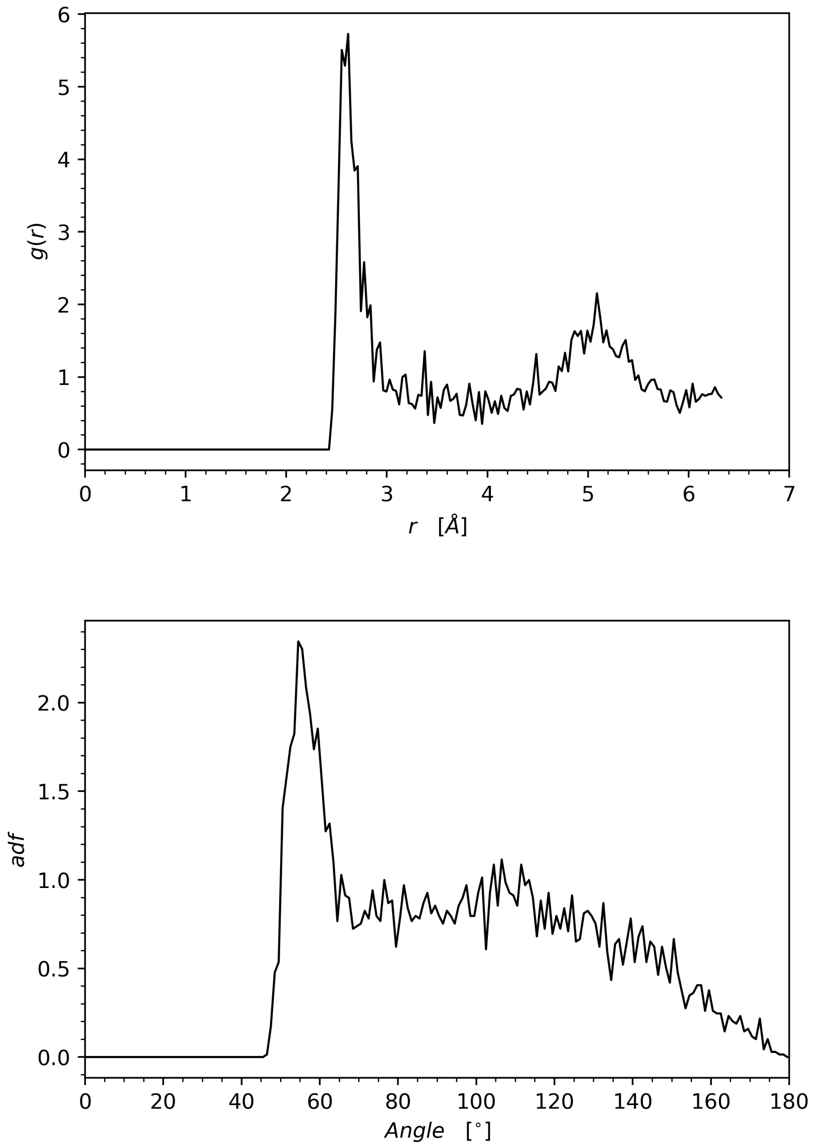


FIG. 3. Radial (a) (upper panel) and angular (b) (lower panel) distribution function (Ge-Ge-Ge bond angles) of the amorphous structure created by static compression of the clathrate $Ge_{136}$ at $p = 350$ kbar.

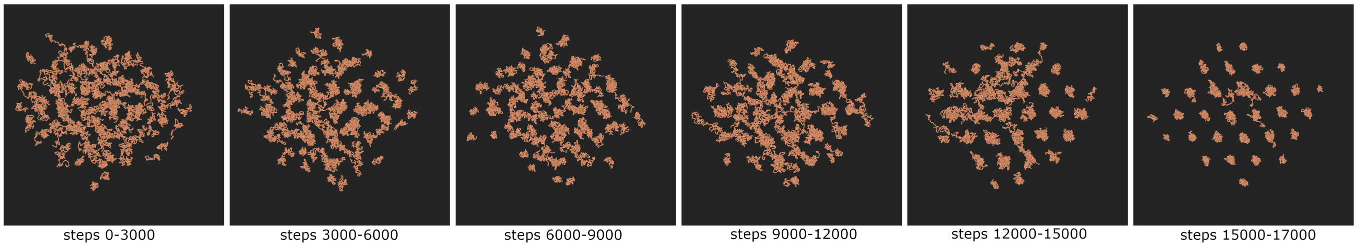


FIG. 4. Atomic trajectories in selected time intervals showing the creation of crystalline structure at $p = 100$ kbar and $T = 300$ K.

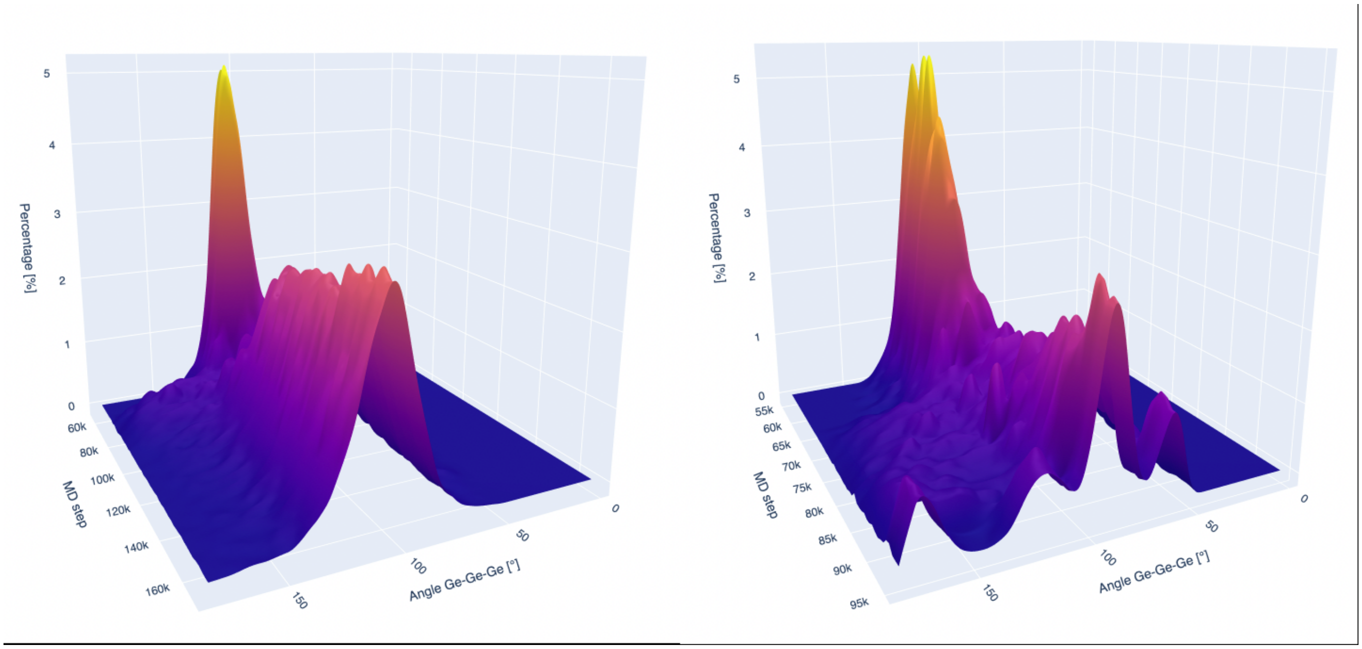


FIG. 5. Evolution of the distribution of the Ge-Ge-Ge bond angles of the system during amorphization of the clathrate at 50 kbar and subsequent decompression to 11 kbar (left panel) and 20 kbar (right panel).
